# Supplementary material for: CARMA: Contention-aware Auction-based Resource Management in Architecture
Source: arXiv:1710.00073 source file (2018-07-19)
Supplement: Supplementary file 1 [file Appendix.tex]

\section{Appendix}
In this section, we show that when the number of applications is large enough, CARMA is strategy-proof, such that no application can get more utilization by bidding more or less than the true value of the resource. 
\vspace{0.5\baselineskip}
\begin{proof}[Proof of Theorem 1]% \ref{thm:neat}]
Suppose all other players bidding strategy is to choose $\frac{n-m}{n-m+1}v_i$. Since the bidding values were derived uniformly in $[0, 1]$ all bids have the same probability. Therefore, if we consider the first player's expected utility to find its best response, we have:
%%%%%%%%%%%%%%%%%%%%%%%%%%%%%%%%%%%%%%%%%%%%%%%%%%%%%%%%%%%%%%%%%%%%%%%%%
\begin{small}
\begin{equation}
%\begin{IEEEeqnarray}{rCl}
E[u_1] = \int_0^1  .... \int_0^1 \! (v_1 -b_1) \, \mathrm{d}u_2 \mathrm{d}u_3 ... \mathrm{d}u_{n-m} .  
%\end{IEEEeqnarray}
\end{equation}
\end{small}
%%%%%%%%%%%%%%%%%%%%%%%%%%%%%%%%%%%%%%%%%%%%%%%%%%%%%%%%%%%%%%%%%%%%%%%%%
The following integral breaks into two part where the first player wins the auction or not. 
%%%%%%%%%%%%%%%%%%%%%%%%%%%%%%%%%%%%%%%%%%%%%%%%%%%%%%%%%%%%%%%%%%%%%%%%%
%\begin{IEEEeqnarray}{rCl}
%E[u_1] = \int_0^{b_1}  .... \int_0^{b_1} \! (v_1 -b_1) \, \mathrm{d}u_2 \mathrm{d}u_3 ... %\mathrm{d}u_{n-m}  \\
%+ \int_{b_1}^1  .... \int_{b_1}^1 \! (v_1 -b_1) \, \mathrm{d}u_2 \mathrm{d}u_3 ... \mathrm{d}%u_{n-m}\nonumber 
%\end{IEEEeqnarray}
%%%%%%%%%%%%%%%%%%%%%%%%%%%%%%%%%%%%%%%%%%%%%%%%%%%%%%%%%%%%%%%%%%%%%%%%%
\begin{small}
\begin{align}
E[u_1] = \int_0^{\frac{n-m+1}{n-m}b_1}  .... \int_0^{\frac{n-m+1}{n-m}b_1} \! (v_1 -b_1) \, \mathrm{d}u_2 ... \mathrm{d}u_{n-m}  \nonumber \\
 + \int_{\frac{n-m+1}{n-m}v_1}^1  .... \int_{\frac{n-m+1}{n-m}v_1}^1 \! (v_1 -b_1) \, \mathrm{d}u_2 \mathrm{d}u_3 ... \mathrm{d}u_{n-m} 
\end{align}
\end{small}
%\begin{equation} \label{eq1}
%\begin{split}
%\end{split}
%\end{equation}
%%%%%%%%%%%%%%%%%%%%%%%%%%%%%%%%%%%%%%%%%%%%%%%%%%%%%%%%%%%%%%%%%%%%%%%%%
The second part of the integrals is the term where the first player doesn't win the auction. Therfore, the expected payoff of player 1 is equal with:
%%%%%%%%%%%%%%%%%%%%%%%%%%%%%%%%%%%%%%%%%%%%%%%%%%%%%%%%%%%%%%%%%%%%%%%%%
%\begin{IEEEeqnarray}{rCl}
%E[u_1] = \int_0^{b_1}  .... \int_0^{b_1} \! (v_1 -b_1) \, \mathrm{d}u_2 \mathrm{d}u_3 ... %\mathrm{d}u_{n-m}  \\
%= {({b_1}) }^{n-m} (v_1 -b_1). \nonumber 
%\end{IEEEeqnarray}
%%%%%%%%%%%%%%%%%%%%%%%%%%%%%%%%%%%%%%%%%%%%%%%%%%%%%%%%%%%%%%%%%%%%%%%%%
\begin{small}
\begin{align}
%\begin{IEEEeqnarray}{rCl}
E[u_1] =\int_0^{\frac{n-m+1}{n-m}b_1}  .... \int_0^{\frac{n-m+1}{n-m}b_1} \! (v_1 -b_1)  \mathrm{d}u_2 ... \mathrm{d}u_{n-m} \nonumber \\
= {(\frac{n-m+1}{n-m} b_1) }^{n-m} (v_1 -b_1).  
%\end{IEEEeqnarray}
\end{align}
\end{small}
%%%%%%%%%%%%%%%%%%%%%%%%%%%%%%%%%%%%%%%%%%%%%%%%%%%%%%%%%%%%%%%%%%%%%%%%%
Differentiating with respect to $b_1$ the optimal bid for player one is derived as follows:
%%%%%%%%%%%%%%%%%%%%%%%%%%%%%%%%%%%%%%%%%%%%%%%%%%%%%%%%%%%%%%%%%%%%%%%%%
%\begin{equation}
%\frac{\partial}{\partial b_1} ( {({b_1}) }^{n-m} (v_1 -b_1))=0.
%\end{equation}
%%%%%%%%%%%%%%%%%%%%%%%%%%%%%%%%%%%%%%%%%%%%%%%%%%%%%%%%%%%%%%%%%%%%%%%%%
\begin{small}
\begin{equation}
\frac{\partial}{\partial b_1} ( {(\frac{n-m+1}{n-m} b_1) }^{n-m} (v_1 -b_1))=0.
\end{equation}
\end{small}
%%%%%%%%%%%%%%%%%%%%%%%%%%%%%%%%%%%%%%%%%%%%%%%%%%%%%%%%%%%%%%%%%%%%%%%%%
Which gives us the optimal bid for each player:
\begin{small}
\begin{equation}
\Rightarrow b_1= \frac{n-m}{n-m+1}v_1
\end{equation}
\end{small}
\end{proof}
